# Supplementary material for: Separations in the Representational Capabilities of Transformers and Recurrent Architectures
Source: arXiv:2406.09347 source file (2024-06-13)
Supplement: Supplementary file 1 [file roadmap.tex]

\section*{Roadmap}
The appendix is organized as follows.
\begin{itemize}
    \item In Section~\ref{app:clarifications}: \textit{Clarifications}, we discuss clarifications related to some natural questions related to our results.
    \item In Section~\ref{app:prelims}: \textit{Preliminaries}, we discuss basic tools in communication complexity used in our work, provide details of finite precision setting, and introduce a key technical tool used in our paper.
    \item In Section~\ref{app:posindex}: \textit{Index Lookup Task}, we provide the details of the proofs for results (Theorems \ref{thm:tf_posret_main} and \ref{thm:rnn_posret_main}) related to the Index Lookup task.
    \item In Section~\ref{app:comm-compl-1-layer}: \textit{Lower Bounds for 1-layer Transformers}, we provide the details of the proof of the result (Theorem~\ref{thm:one-layer-commun_mainPaper}) regarding the communication protocol for one-layer Transformers which forms the basis of the lower bound results for the model.
    \item In Section~\ref{app:dyck}: \textit{Dyck with Bounded Depths}, we provide the proof for the lower bound on the communication complexity of bounded Dyck languages which leads to the lower bound on the size of one-layer Transformers.
    \item In Section~\ref{app:bool}: \textit{Transformers and Boolean functions}, we discuss the constructions of two-layer Transformers for computing the Equality functions as well as a more general class of Boolean functions. We also discuss the lower bounds for one-layer Transformers and recurrent models such tasks. Lastly, we discuss the difficulty of deriving similar lower bounds for two-layer Transformers.
    \item In Section~\ref{app:nn}: \textit{Nearest Neighbors and Associative Recall}, we provide the details of the proof for the upper bound result for two-layer Transformers (Theorem~\ref{thm:tf_nn_main}) and lower bound result for recurrent models (Theorem~\ref{thm:rnn_nn_lower_main}) for implementing the nearest neighbor task.
    \item In Section~\ref{app:experiments}: \textit{Empirical Analysis}, we provide the details about the implementation and discuss additional experiments related to the Index Lookup task and the string Equality task.
\end{itemize}
